# Supplementary material for: Hybridized Frequency Combs in Multimode Cavity Electromechanical System
Source: arXiv:2203.06536 ancillary file (2022-03-12)
Supplement: Supplementary file 1 [file Supplementary_Materials.pdf]

# Supplementary Materials for " Hybridized Frequency Combs in Multimode Cavity Electromechanical System "

Sishi Wu,[1] Yulong Liu,[2,*] Qichun Liu,[2] Shuai-Peng Wang,[1] Zhen Chen,[2] and Tiefu Li[3,2,†]

[1]*Quantum Physics and Quantum Information Division, Beijing Computational Science Research Center, Beijing 100193, China*

[2]*Beijing Academy of Quantum Information Sciences, Beijing 100193, China*

[3]*School of Integrated Circuits and Frontier Science Center for Quantum Information, Tsinghua University, Beijing 100084, China*

## I. EXPERIMENTAL SETUP

As is introduced in the main text, our sample is composed of a mechanically compliant capacitor chip and a 3D cavity. While 3D cavity electromechanical system avoids complexity induced by material instability under strong drive, the electromechanical coupling and cooperativity are comparatively weaker. Therefore, we apply mechanically compliant capacitor in the design.

In contrast to direct galvanic coupling through indium foil extrusion, the wireless connection between mechanical compliant capacitor and 3D cavity can effectively avoid any unexpected external force disturbance and stress uneven distribution for the SiN membrane. The coupling capacitance is huge compared to the other capacitors in our system. These two large capacitors are connected in series in the circuit. In principle, our circuit model is equivalent to a galvanic connection, enlarging single photon coupling strength while minimizing stress disturbance for SiN membrane.

The electric field distribution is analysed by finite element method. As is shown in Fig. S1, the 40 mm $\times$ 8 mm $\times$ 14 mm sized electric field in the 3D cavity is tailored by a 11 mm $\times$ 8 mm $\times$ 0.43 mm sized capacitor chip, resulting in expected characteristic frequency of 5.95 GHz. The cavity field changes from a quasi evenly distribution to a chip focused one. Further introducing a 5 mm $\times$ 5 mm $\times$ 0.5 mm sized mechanical part, the resonant frequency is tuned to be 5.31 GHz. Capacitive coupling between on chip antenna and membrane back electrode enhances cooperation between electric field and mechanical motion.

To bring the expectation down to earth, there are several fabrication tricks adopted. Packaging material to glue and define the gaps between the upper SiN and lower antenna chips is chosen to be epoxy resin pillars after rounds of applicability tests, due to its outstanding performances, such as introducing negligible dissipation for cavity and mechanical modes. Even at millikelvin temperature, the epoxy based encapsulation can still maintain a narrow gap for the mechanically compliant capacitor and will not change the stress distribution of the SiN membrane. In addition to avoiding stress changes caused by packaging materials, we should also take care of the Coulomb force caused by charge accumulation. For the bottom antenna chips, we use high-resistance silicon as its substrate to match the shrinkage to the SiN chips during the cooling process. Note that any accumulated charge

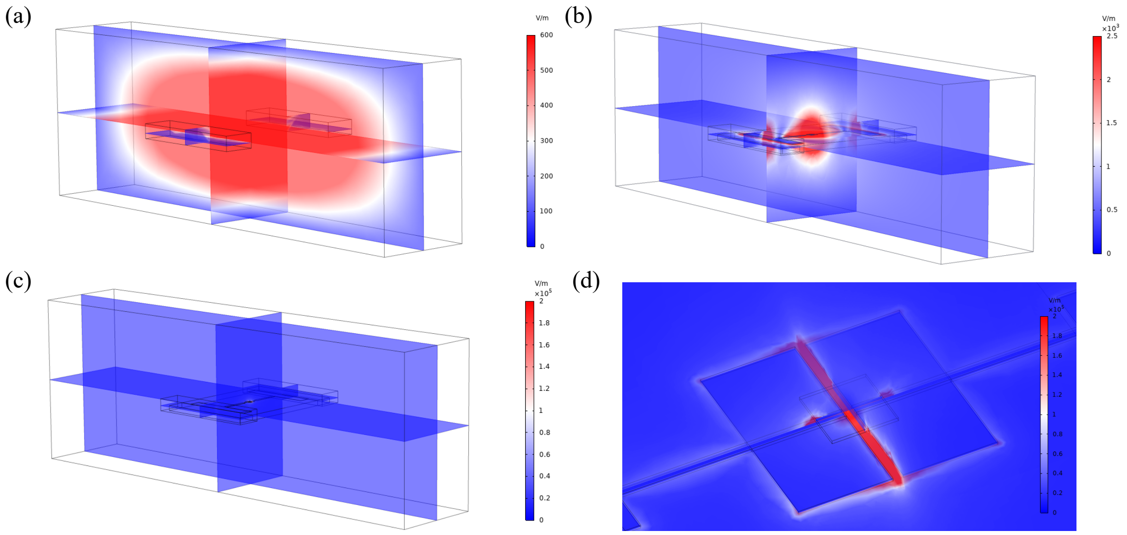


FIG. S1. Simulation of the intra cavity electric field. (a) Case of empty rectangular cavity without embedded chip. (b) Case of capacitor chip embedded cavity without mechanical part. (c) Case of mechanically compliant capacitor chip embedded cavity. (d) Zoom in of the mechanical part in subfigure(c).

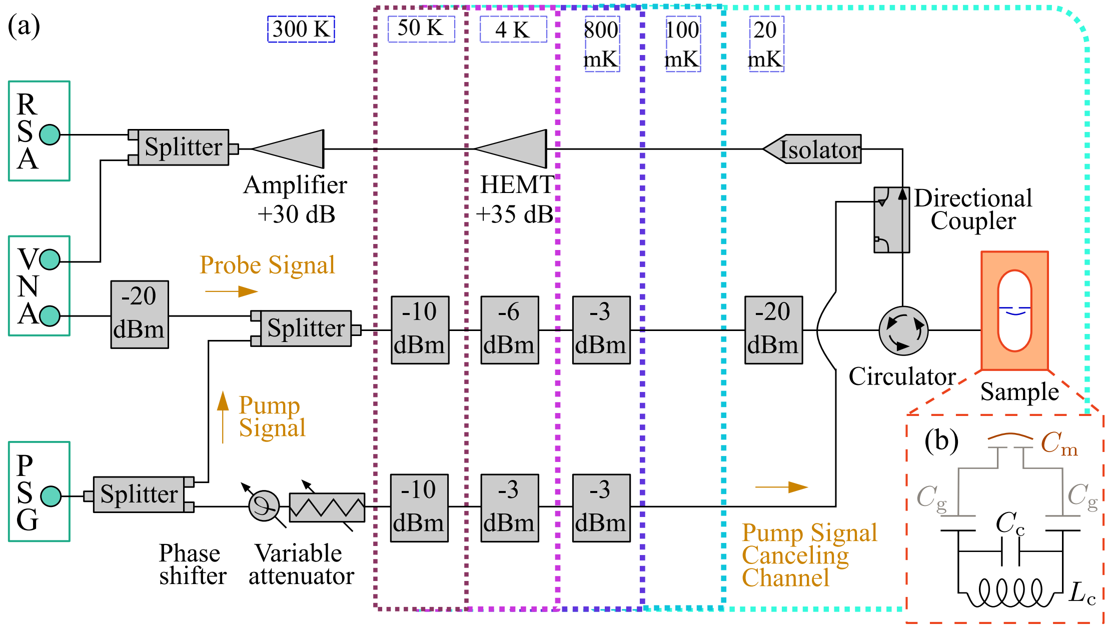


FIG. S2. (a) Experimental setup. Sideband pumps are injected to study nonlinear cavity dynamics. Heterodyne reflection readout is adopted to observe frequency comb formation. (b) Lumped-element circuit model of the electromechanical system. Brown arc represents mechanical oscillating element.

under the membrane will harass the uniform stress distribution and thus greatly broaden the mechanical linewidth. Compared to the insulating substrate such as sapphire or quartz, silicon substrate can efficiently avoid charge accumulation. In addition, The area of the silicon wafer, directly under the SiN film, is covered by Al film to further remove the charges.

Detailed cryogenic setup, as well as room temperature microwave devices are presented in Fig. S2(a). Attenuators in three input channels (marked by orange arrows) are used to reduce background noise. Circulator, isolator and directional couplers help avoid back reflections. Network analyzer (VNA) is mainly used for preliminary characterization. Spectrum Analyzer (RSA) is used for more specifical spectrum detection, including both frequency and time domain features. Signal components involved in the experiment includes microwave range resonant frequency of the cavity, and signal generator (PSG) emitted pump frequency. Both amplitude and frequency of the pump will manipulate the cavity fields. Change of the cavity field can influence the motion of embedded membrane, which in turn changes cavity frequency and thus account for cavity photon number fluctuation. Such feedback regime stimulates Kerr-like nonlinearity. Effective circuit model of the sample is presented in Fig. S2(b).

Based on the channel for probe signal injection, basic characteristic parameters of the system are obtained. Fig. S3(a) refers to the unpumped reflection of the 3D cavity, which characterize the resonant frequency and damping rate. The detection is done by VNA. Fig. S3(b-c) refers to the power spectral density of the two mechanical modes, which are obtained when the cavity is near resonantly pumped, with detunings in the order of targeted mechanical mode frequency. The detection is done by RSA via IQ mixing based frequency down conversion. Relative frequency $\Omega_{\mathrm{ref1}}$ and $\Omega_{\mathrm{ref2}}$ refer to raw frequency with offset $\Omega_c + \Omega_{m1}$ and $\Omega_c + \Omega_{m2}$. Pump power for Fig. S3(a,b,c) are −60 dBm, −70 dBm, and −30 dBm respectively.

Combined with bare cavity measurement (11.4 GHz, 100 KHz), characterising measurements help certificate effective parameters of the circuit model [S1], including cavity inductance $L_c = 6.17$ fH, $C_c = 31.8$ nF, $C_g = 23.7$ nF, and $C_m(0) = 13.2$ nF. Based on numerical simulation and experimental measured single coupling strength, we can construct mechanical mode induced negative cavity frequency shift as $G_1/(2\pi) = 2.43$ THz/m, $G_2/(2\pi) = 0.53$ THz/m, and effective mass as $m_{\mathrm{eff}} = 0.27$ fg.

Except for basic parameters, pump power dependency of the optomechanical system is also studied. Optomechanically induced transparency for each mode is observed, which certificates activity of mechanical motions. Fig. S3(d,f) illustrate changed amplitude of cavity reflection under varied pump power, with detuning set to be targeted mechanical mode frequency. $\Delta_{sc}$ labelled here represents detuning of probe signal ($\Omega_s$) from the cavity resonant frequency ($\Omega_c$). Gray dash lines refer to the pump power condition picked for Fig. S3(e,g), which illustrate the detailed spectrum when cavity transparency happen. Embedded subfigures in Fig. S3(e,g) are zoom in plots for the dash boxes. Circled dots refer to measured data and the black lines are Lorentzian fitting results.

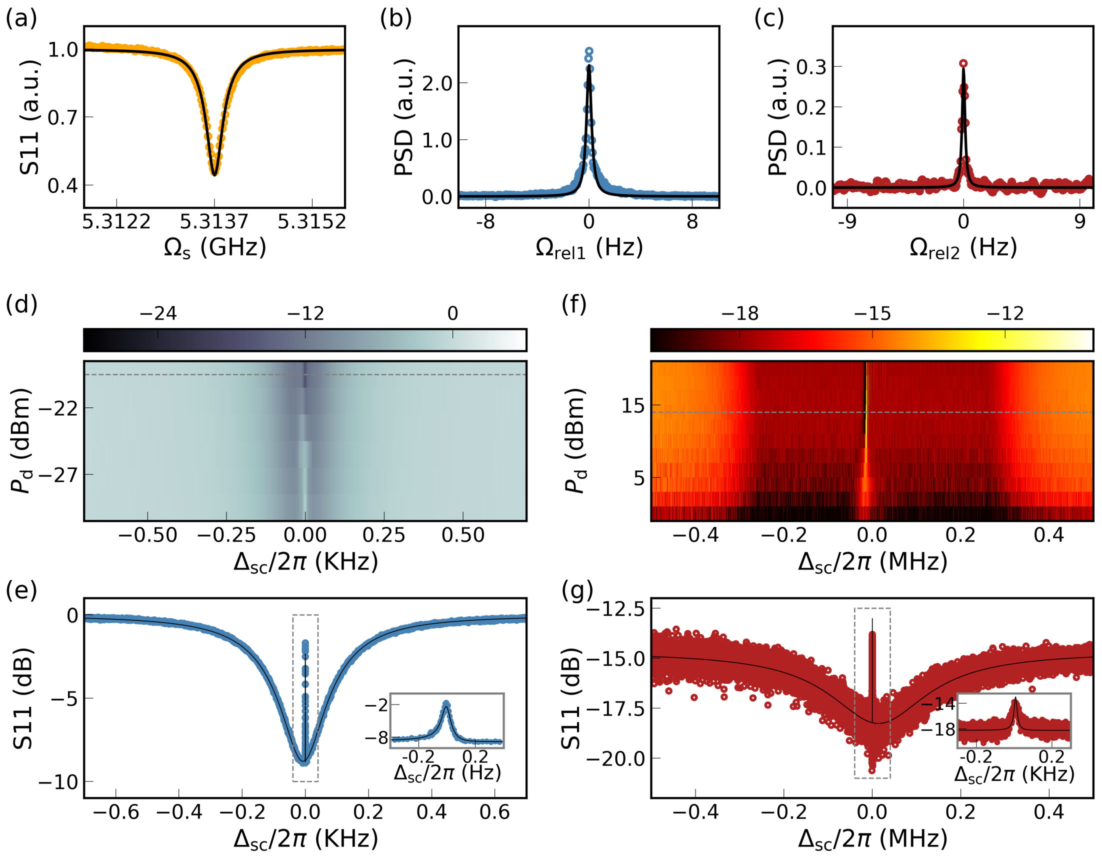


FIG. S3. (a) Measured reflection of the 3D cavity. (b-c) Measured power spectral density of the first and second mechanical mode. (d-e) First mechanical mode induced cavity transparency. (f-g) Second mechanical mode induced cavity transparency.

## II. SINGLE PHOTON COUPLING STRENGTH

While Fig. S3(a-c) already give characteristic parameters, yet the value is not accurate enough because of the thermal excitation on the mechanical modes. Exact single photon coupling strength can be derived from comparing spectrum of the thermomechanical sideband with the spectrum of a reliable calibration tone under reliable temperature, where thermomechanical sideband is thermally determined.

Therefore, in order to calibrate phonon number in the two modes, we firstly apply heating source to vary the dilution fridge temperature, and observe spectral change of the mechanical modes. As is shown in Fig. S4(a) and (d), dependency of spectrum area on temperature becomes linear above $T \approx 50$ mK, while the dilution fridge temperature is typically around 20 mK without heating source. Consequently, we chose the environment condition of 55 mK to measure single photon coupling strengths.

By studying the spectral feature of each mechanical mode, when a calibration tone and a cavity pump tone are injected, we experimentally derive $g_1$ and $g_2$. The calibration is set to be slightly detuned from $\Omega_c + \Omega_{mj}$, and outside the mechanical linewidth. As a result, two output signals would be observed by the RSA, including thermomechanical sideband created by a resonant pump [see Fig. S4(b) and (e)] and calibration tone [see Fig. S4(c) and (f)]. Taking calibration tone as a reference, the single photon coupling strengths can be concludes as [S2, S3]

$$g_j = \frac{r}{2n_m}\left(\frac{\kappa}{\kappa_e}\right)^2\left(\Omega_{mj}^2 + \frac{\kappa^2}{2}\right)\frac{P_{SB}}{P_{cali}}\,, \tag{S.1}$$

where $r$ represents input power ration between injected calibration tone and cavity pump tone for the corresponding cases. $n_m = k_b T/(2\pi\hbar\Omega_{mj})$, representing phonon number under $T = 55$ mK, with $k_b$ referring to Boltzmann constant. $P_{SB}$ and $P_{cali}$ represent the detected power of the thermomechanical sideband and calibration tone, measured at the end of the output chain by

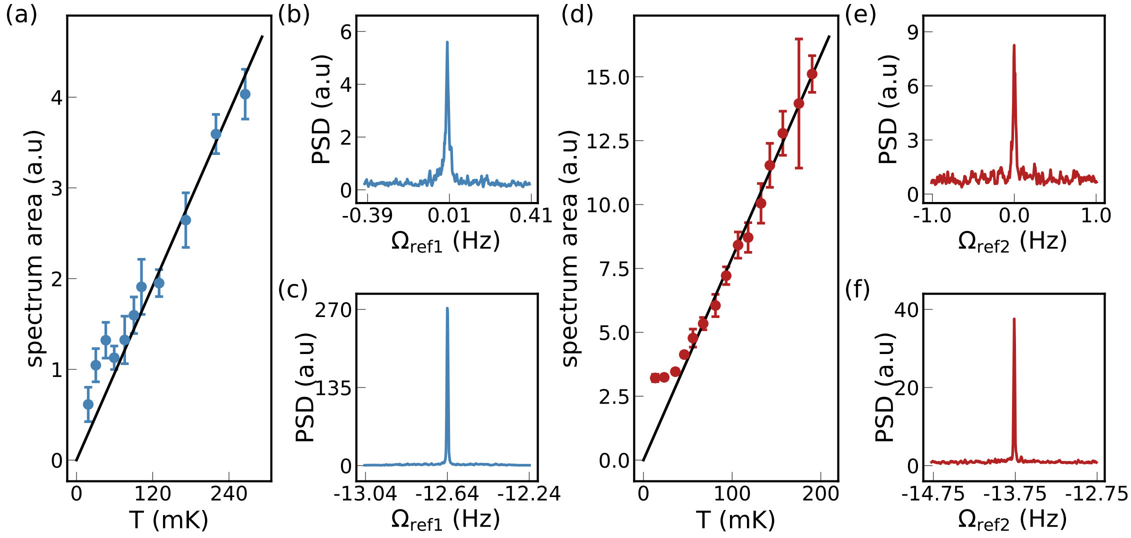


FIG. S4. (a,d) Temperature dependency of spectrum area for the first (blue data) and second (red data) mechanical mode. Black lines are linear fitting. Errorbars come from repeated measurements for a fixed heating source setting. (b,e) Detected spectrum of the first and second mechanical mode mediated thermomechanical sideband. (c,f) Detected spectrum of the first and second mechanical mode targeted calibration tone. Note the xticks for (b,c,e,f) only serve as a relative value.

the RSA. Their ratio are indeed the ratio of area under the mechanical peak to the area under the modulation peak. As a result, we can conclude $g_1 = 0.49$ Hz, and $g_2 = 0.07$ Hz.

## III. THRESHOLD OF STABILITY

Threshold of intra-cavity field stability can be understood as solvability of the pumped cavity field, which can be treated seperately in classical steady state and small fluctuating term, i.e., $a = \bar{a} + \delta a$. Ignoring small back-action of the radiation pressure force, amplitude of classical steady state is governed by $\bar{a} = \sqrt{\kappa_e} S_{\rm in}/(-i\Delta_{\rm dc} + \kappa/2)$. Solvability then counts on the small fluctuation term, or say self-oscillation harmonics $\delta a$.

For simplification, since $g_1 \gg g_2$, we can separately analyse instability mediated by single mechanical mode, which is well approximation when the pump is not strong enough and does not match the sum of cavity frequency and second mechanical mode frequency. Therefore, only cavity and first mechanical mode related terms are considered initially. With consideration of Laplace transformation and dynamics of classical mechanical motion $\ddot{x}_{\rm j} + \gamma_{\rm j}\dot{x}_{\rm j} + \Omega_{\rm mj}^2 x_{\rm j} = \hbar G_{\rm j}|a|^2/m_{\rm j}$, requirements for solvability are thus given as [S4]

$$3\chi_1^2 + 4\Delta_{\rm dc}\chi_1 + \Delta_{\rm dc}^2 + \frac{\kappa^2}{4} > 0\,, \tag{S.2a}$$

$$\chi_1^4 + d_1\chi_1^3 + d_2\chi_1^2 + d_3\chi_1 + d_4 > 0\,, \tag{S.2b}$$

where mechanical mode induced cavity frequency shift $\chi_1 \equiv 2g_1^2|\bar{a}|^2/\Omega_{\rm m1}$, and coefficients are defined as

$d_1 \equiv 4\Delta_{\rm dc}$,

$d_2 \equiv \gamma_1\kappa + 6\Delta_{\rm dc}^2 + \gamma_1^2 - 6\Omega_{\rm m1}^2 + \frac{\kappa^2}{2} - 2\gamma_1\Omega_{\rm m1}^2/\kappa - 2\Omega_{\rm m1}^2\kappa/\gamma_1$,

$d_3 \equiv \Delta_{\rm dc}(2\gamma_1\kappa + 4\Delta_{\rm dc}^2 + 2\gamma_1^2 - 8\Omega_{\rm m1}^2 + \kappa^2 - 2\gamma_1\Omega_{\rm m1}^2/\kappa - 2\Omega_{\rm m1}^2\kappa/\gamma_1)$,

$d_4 \equiv \Delta_{\rm dc}^2(\Delta_{\rm dc}^2 + \gamma_1^2 + \gamma_1\kappa - 2\Omega_{\rm m1}^2 + \frac{\kappa^2}{2}) + \frac{\gamma_1^2\kappa^2}{4} + \gamma_1\Omega_{\rm m1}^2\kappa + \frac{\gamma_1\kappa^3}{4} + (\Omega_{\rm m1}^2 + \frac{\kappa}{4})^2$.

As is shown in Fig. S5, primary instability occurs around $\Delta_{\rm dc} = \Omega_{\rm m1}$ at $-75$ dBm (31.6 picowatt), where the lower sideband

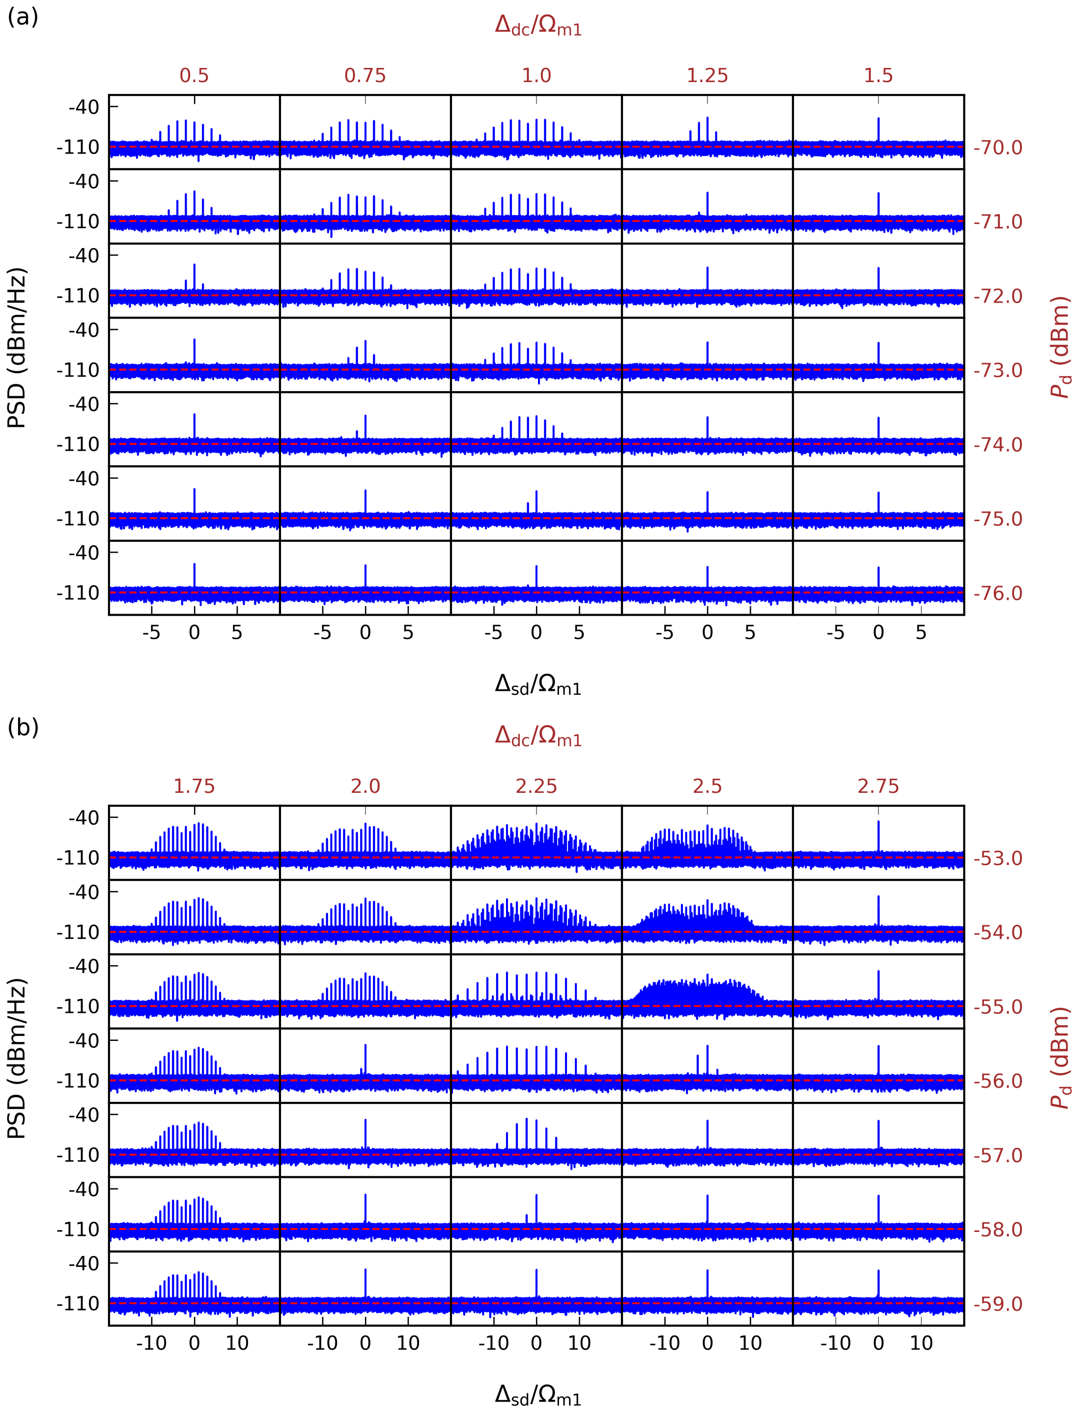


FIG. S5. Detailed primary formation of frequency combs around $\Delta_{dc} = \Omega_{m1}$ and $\Delta_{dc} = \Omega_{m2}$. Red labels refer to pump conditions, black labels refer to detected parameters. Note that x-axis span for the two graphs is different.

is suppressed, and the total optomechanical system is most efficiently pumped. The theoretical threshold analysis matches well with the experimental observation. Similarly, single second mechanical mode based regime explains appearance of combs for pump detuning close to the sum of cavity frequency and second mechanical mode frequency. As is indicated by Fig. S3(d,f), mechanical mode frequency keeps unchanged along increased pump power within the detected range, which leads to stable tooth spacing for frequency comb spectra.

Combined with calibration of single photon coupling strength measurement, instability threshold criterion, i.e., Eq. S.2a and

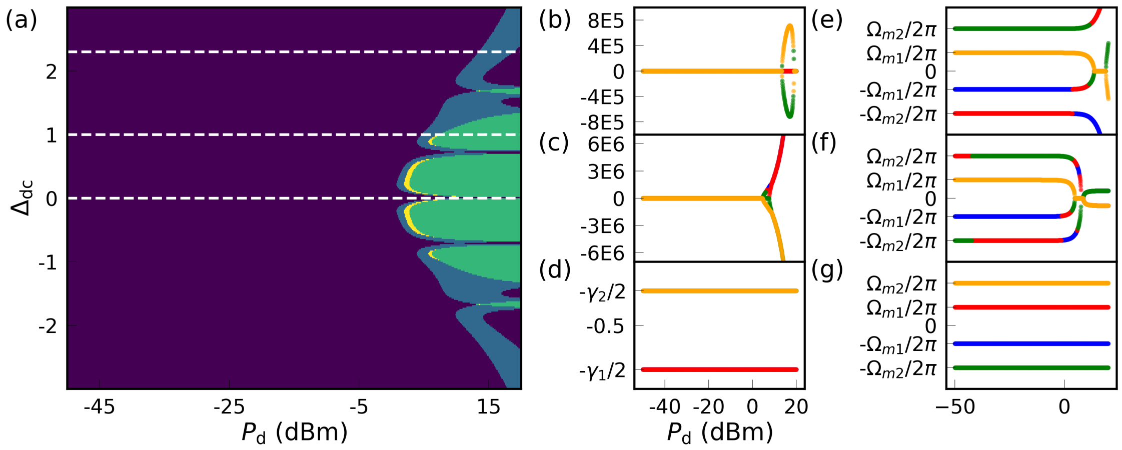


FIG. S6. Pump condition dependent eigenvalues of the coefficient matrix. (a) The color indicates different types of the eigenvalues. (b-d) Zoom in of pump power dependent decay rate for fixed detuning at $\Delta_{dc}/\Omega_{m1} = 0,\ 1,\ 2.3$. (e-f) Zoom in of pump power dependent rotating frequency for fixed detuning at $\Delta_{dc}/\Omega_{m1} = 0,\ 1,\ 2.3$. There are four eigenvalues, and are colored in different colors.

S.2a, gives the corresponding threshold plotted as dash lines in Fig. 3 in the main text. It is worth noting that such theoretical analysis only predicts the timing of comb formation, not explain of spectral behaviour for self-organization beyond the instability threshold.

## IV. EFFECTIVE PHONON-PHONON COUPLING

Although two mechanical modes are not directly coupled, cavity field enables their effective coupling [S5]. In the perspective of Hamiltonian, photon-phonon coupling can be written as

$$H_{cm}/\hbar = \sum_{j=1,2} g_j(b_j + b_j^\dagger)(\bar{a}^*\delta a + \bar{a}\delta a^\dagger) \tag{S.3}$$

where the foot label 'cm' in $H_{cm}$ refers to interaction between cavity and membrane. Small terms like $\delta a^\dagger\delta a$ are dropped. $H_{cm}$ explains averaged photon number dependent mechanical motion, and the consequent cavity field fluctuation. Therefore, effective photon-phonon coupling strength for the $j$-th mechanical mode can be defined as $I_j = g_j\bar{a}$. Subsequently, phonon-phonon coupling via cavity field can be written as

$$H_{mm}/\hbar = \frac{J_r}{2}(b_1^\dagger b_2 + b_1 b_2^\dagger) + \frac{J_b}{2}(b_1^\dagger b_2^\dagger + b_1 b_2) \tag{S.4}$$

where the foot label 'mm' in $H_{mm}$ refers to interaction between two membrane modes, $J_r = \mathrm{Im}\{I_1 I_2(\kappa - 2i\Delta_{dc})/[\kappa^2 + (\Omega_{m1} + \Omega_{m2})^2/4 - \Delta_{dc}{}^2 - i\kappa\Delta_{dc}]\}$, which can result in phonon state transfer, and $J_b = \mathrm{Im}\{I_1 I_2(\kappa - 2i\Delta_{dc})/[\kappa^2 + (\Omega_{m1} - \Omega_{m2})^2/4 - \Delta_{dc}{}^2 - i\kappa\Delta_{dc}]\}$, which can result in parametric conversion. Such virtual coupling explains mixing procedure on one mechanical mode mediated frequency comb that causes additional sets detuned by the order of another mechanical mode, and cascadedly, creates hybridized spectrum, which is plotted and analysed detailly in the main text.

The total Hamiltonian in the effective coupling picture yields equations of motion as

$$\frac{\partial}{\partial t}\begin{pmatrix} b_1 \\ b_1^\dagger \\ b_2 \\ b_2^\dagger \end{pmatrix} = \begin{pmatrix} -(i\Omega_{m1} + \frac{\gamma_1}{2}) & 0 & -\frac{i}{2}J_r & -\frac{i}{2}J_b \\ 0 & +(i\Omega_{m1} - \frac{\gamma_1}{2}) & \frac{i}{2}J_b & \frac{i}{2}J_r \\ -\frac{i}{2}J_r & -\frac{i}{2}J_b & -(i\Omega_{m2} + \frac{\gamma_2}{2}) & 0 \\ \frac{i}{2}J_b & \frac{i}{2}J_r & 0 & +(i\Omega_{m2} - \frac{\gamma_2}{2}) \end{pmatrix}\begin{pmatrix} b_1 \\ b_1^\dagger \\ b_2 \\ b_2^\dagger \end{pmatrix}, \tag{S.5}$$

which show oscillating dependency of one mechanical mode on another. Eigenvalues of the coefficient matrix under varied pump condition can be sorted into four types. As is shown in Fig. S6(a), the dark blue region refers to all negative eigenvalues. Blue

region refers to three negative eigenvalues and one positive eigenvalue. Yellow region refers to one negative eigenvalue and three positive eigenvalues. Green region refers to two negative eigenvalue and two positive eigenvalues.

Within the dark blue region of pump condition, pure states of each mechanical mode are exactly eigenmodes of their virtually coupled system. Therefore, their accordingly mechanical motion is reasonable to be expressed as $b_{\mathrm{j}} = B_{\mathrm{j}} e^{-i(\Omega_{\mathrm{mj}} t+\varphi_0)}$, and $B_{\mathrm{j}}$ slowly decays in a rate of $\kappa/2$. Taking initial displacement of the membrane as 0, $\varphi_0$ can be regarded as $\pi/2$. It can be inferred that for large pump power, evolution of two mechanical mode are no longer independent with each other but having energy exchanging.

## V. MULTI MECHANICAL MODE COMPETITION

While theoretical analysis on threshold of stability serves as a guide of timing, the explain of spectral behaviour for frequency combs can be referred from Bessel functions based on Jacobi-Anger expansion, i.e., $e^{i\xi\cos\phi} = \sum_{k=-\infty}^{\infty} i^k J_k(\xi) e^{ik\phi}$. Substituting trial solution of membrane motion as $b_j = B_j e^{-i(\Omega_{mj}t+\pi/2)}$, cavity field can be written as [S6–S8]

$$\begin{aligned} a &= \sqrt{\kappa_{\mathrm{e}}} S_{\mathrm{in}} \exp\{i[\Delta_{\mathrm{dc}} t - \sum_{j=1,2} \xi_{\mathrm{j}} \cos(\Omega_{\mathrm{mj}} t)] - \frac{\kappa}{2} t\} \cdot \int_{-\infty}^{t} \exp\{-i[\Delta_{\mathrm{dc}} \tau - \sum_{j=1,2} \xi_{\mathrm{j}} \cos(\Omega_{\mathrm{mj}} \tau)] + \frac{\kappa}{2}\tau\} d\tau \\ &= \sqrt{\kappa_{\mathrm{e}}} S_{\mathrm{in}} \exp[-i \sum_{j=1,2} \xi_{\mathrm{j}} \cos(\Omega_{\mathrm{mj}} t)] \cdot \sum_{k,l=-\infty}^{\infty} i^{k+l} \frac{e^{ik\Omega_{\mathrm{m1}} t} e^{il\Omega_{\mathrm{m2}} t} J_k(\xi_1) J_l(\xi_2)}{\kappa/2 - i(\Delta_{\mathrm{dc}} - k\Omega_{\mathrm{m1}} - l\Omega_{\mathrm{m2}})}, \end{aligned} \tag{S.6}$$

where $J_n(\xi_{\mathrm{j}})$ represents the n-th order Bessel function of the first kind, and $\xi_{\mathrm{j}} = 2g_j B_{\mathrm{j}}/\Omega_{\mathrm{mj}}$. Therefore,

$$|a|^2 = \kappa_{\mathrm{e}} S_{\mathrm{in}}^2 \sum_{k,l,s,q=-\infty}^{\infty} i^{s+q} \frac{e^{is\Omega_{\mathrm{m1}} t + iq\Omega_{\mathrm{m2}} t} J_k(\xi_1) J_l(\xi_2) J_{k-s}(\xi_1) J_{l-q}(\xi_2)}{[\kappa/2 - i(\Delta_{dc} - k\Omega_{m1} - l\Omega_{m2})]\{[\kappa/2 + i[\Delta_{\mathrm{dc}} - (k-s)\Omega_{\mathrm{m1}} - (l-q)\Omega_{\mathrm{m2}}]\}}, \tag{S.7}$$

whereas magnitude of the first order comb tooth individually mediated by the j-th mechanical mode is proportional (influenced by the transmission characteristics along output channel) to

$$P_1^{\mathrm{t1}} = \hbar(\Omega_{\mathrm{c}} + \Omega_{\mathrm{m2}}) \sum_{k,l=-\infty}^{\infty} i \frac{\kappa_{\mathrm{e}}^2 S_{\mathrm{in}}^2 J_k(\xi_1) J_{k-1}(\xi_1) J_l^2(\xi_2)}{[\kappa/2 - i(\Delta_{dc} - k\Omega_{m1} - l\Omega_{m2})]\{[\kappa/2 + i[\Delta_{\mathrm{dc}} - (k-1)\Omega_{\mathrm{m1}} - l\Omega_{\mathrm{m2}}]\}}, \tag{S.8a}$$

$$P_2^{\mathrm{t1}} = \hbar(\Omega_{\mathrm{c}} + \Omega_{\mathrm{m2}}) \sum_{k,l=-\infty}^{\infty} i \frac{\kappa_{\mathrm{e}}^2 S_{\mathrm{in}}^2 J_k^2(\xi_1) J_l^2(\xi_2) J_{l-1}^2(\xi_2)}{[\kappa/2 - i(\Delta_{dc} - k\Omega_{m1} - l\Omega_{m2})]\{[\kappa/2 + i[\Delta_{\mathrm{dc}} - k\Omega_{\mathrm{m1}} - (l-1)\Omega_{\mathrm{m2}}]\}}. \tag{S.8b}$$

Note that only signal with power beyond systematic background noise can be observed. Dropping non-resonant terms in Eq. S.7, dynamics of the j-th mechanical mode can be expressed as

$$\dot{B}_{\mathrm{j}} e^{+i\Omega_{\mathrm{mj}} t} + \gamma_{\mathrm{j}} B_{\mathrm{j}}/2 = g_j \kappa_{\mathrm{e}} S_{\mathrm{in}}^2 \sum_{k,l=-\infty}^{\infty} \mathrm{Im}[f_{\mathrm{j}}(k,l)], \tag{S.9}$$

where $f_{\mathrm{j}}$ represents the cavity field contribution to the $j$-th mechanical (anti)damping, and only its imaginary part is taken. Such radiation pressure force determined function can be written as

$$f_1(k,l) = \frac{J_k(\xi_1) J_{k+1}(\xi_1) J_l^2(\xi_2)}{[\kappa/2 - i(\Delta_{\mathrm{dc}} - k\Omega_{\mathrm{m1}} - l\Omega_{\mathrm{m2}})]\{[\kappa/2 + i[\Delta_{\mathrm{dc}} - (k+1)\Omega_{\mathrm{m1}} - l\Omega_{\mathrm{m2}}]\}}, \tag{S.10a}$$

$$f_2(k,l) = \frac{J_k^2(\xi_1) J_l(\xi_2) J_{l+1}(\xi_2)}{[\kappa/2 - i(\Delta_{\mathrm{dc}} - k\Omega_{\mathrm{m1}} - l\Omega_{\mathrm{m2}})]\{[\kappa/2 + i[\Delta_{\mathrm{dc}} - k\Omega_{\mathrm{m1}} - (l+1)\Omega_{\mathrm{m2}}]\}}. \tag{S.10b}$$

For small $\xi_{\mathrm{j}}$, it is reasonable to mainly considering $f_{\mathrm{j}}(0,0)$ for mechanical motion determining functions. Further dropping non-resonant terms, dynamics of the j-th mechanical mode can be simplified as

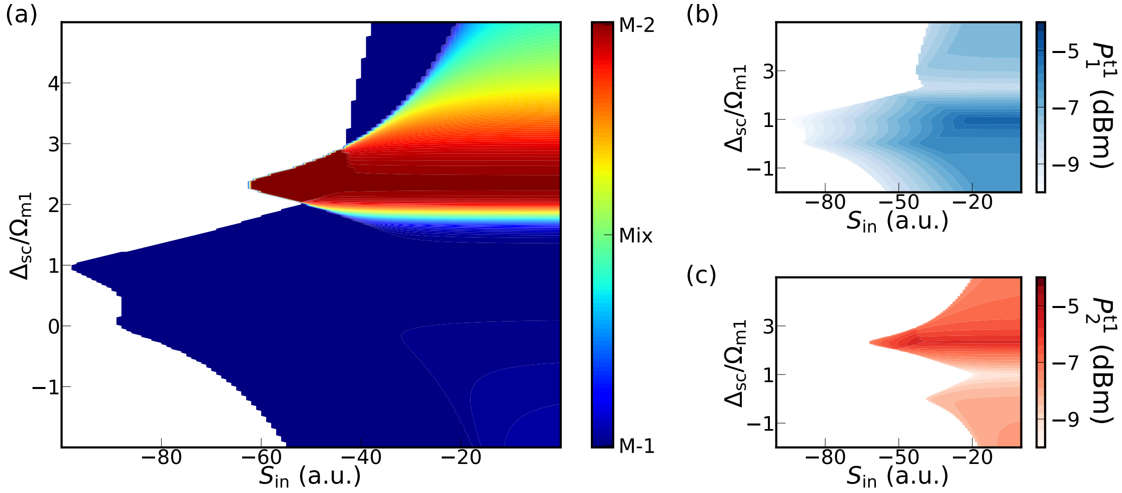


FIG. S7. Calculated motion of multi mechanical modes. (a) Calculated dependency of mode competition results, i.e., $(P_2^{t1} - P_1^{t1})/(P_2^{t1} + P_1^{t1})$, on varied pump power and detuning. (b) Calculated dependency of $P_1^{t1}$ on varied pump power and detuning. (c) Calculated dependency of $P_2^{t1}$ on varied pump power and detuning.

$$\xi_1 = \frac{2g_1^2\kappa_e\kappa S_{in}^2 J_0(\xi_1)J_1(\xi_1)J_0^2(\xi_2)}{\gamma_1(\kappa^2/4+\Delta_{dc}^2)[\kappa^2/4+(\Delta_{dc}-\Omega_{m1})^2]}\ , \tag{S.11a}$$

$$\xi_2 = \frac{2g_2^2\kappa_e\kappa S_{in}^2 J_0^2(\xi_1)J_0(\xi_2)J_1(\xi_2)}{\gamma_2(\kappa^2/4+\Delta_{dc}^2)[\kappa^2/4+(\Delta_{dc}-\Omega_{m2})^2]}\ . \tag{S.11b}$$

For steady state, taking first-order Maclaurin expansion approximation for the Bessel functions, i.e., $J_0(x) \approx 1 - x^2/4$, and $J_1(x) \approx x/2$, the equations can be solved as

$$\xi_1^2 = 4 - 4\sqrt[3]{\frac{\kappa^2/4+\Delta_{dc}^2}{\kappa_e\kappa S_{in}^2}\frac{\gamma_1^2/\gamma_2}{g_1^4/g_2}\frac{[\kappa^2/4+(\Delta_{dc}-\Omega_{m1})^2]^2}{\kappa^2/4+(\Delta_{dc}-\Omega_{m2})^2}}\ , \tag{S.12a}$$

$$\xi_2^2 = 4 - 4\sqrt[3]{\frac{\kappa^2/4+\Delta_{dc}^2}{\kappa_e\kappa S_{in}^2}\frac{\gamma_2^2/\gamma_1}{g_2^4/g_1}\frac{[\kappa^2/4+(\Delta_{dc}-\Omega_{m2})^2]^2}{\kappa^2/4+(\Delta_{dc}-\Omega_{m1})^2}}\ . \tag{S.12b}$$

Substituting the analytical result into Eq. (S.8a-S.8b) and again considering merely $J_0\xi_j$ related terms concludes Fig. S7. While second mechanical mode is most efficiently pumped at $\Delta_{dc} = \Omega_{m2}$, under most pump conditions, the corresponding radiation pressure force on mechanical modes causes the membrane to oscillate on the first mechanical mode [S7]. Even for pump power beyond second mechanical mode mediated cavity field instability, its information is suppressed.

Nature of such mode competition can be seen as modification of $J_1(\xi_1)J_0(\xi_2)$ on $B_1$ and $J_0(\xi_1)J_1(\xi_2)$ on $B_2$. While analytical calculation pointed out the working region of the two mode excitation (around $\Delta_{dc} = \Omega_{m2}$), accumulative effect of series Bessel functions gives another working region around $\Delta_{dc} = \Omega_{m1}/2$, whose spectral features are amply analysed in Fig. 4 of the main text. Within this region, the denominator in Eq. S.10a reaches its minimum value in the nearby parameter range.

Therefore, under most pump conditions, we can take simplification of the cavity field solution as

$$a = \sum_{k=-\infty}^{+\infty} a_k e^{ik\Omega_{\mathrm{mj}}t}\ , \tag{S.13}$$

where $a_k = \sqrt{\kappa_e} S_{\mathrm{in}} \cdot \sum_{n=-\infty}^{+\infty} i^k \frac{J_{k-n}(\xi_j) J_n(-\xi_j)}{\kappa/2 - i(\Delta_{\mathrm{dc}} + n\Omega_{\mathrm{mj}})}$. This equation well describes features of single mechanical mode mediated combs [S9].

As is shown in Fig. 2(b) in the main text, when pump condition is fixed at $\Delta_{\mathrm{dc}} = \Omega_{\mathrm{m1}}$ and $P_{\mathrm{d}} = -29$ dBm and the RSA resolution is fixed to be 20 Hz, resulted frequency spectrum exhibits well suppressed second mechanical mode, with repetition frequency being the first mechanical mode frequency. The total spectrum has 34 comb lines, i.e., bandwidth of 25.7 MHz. Similarly, as is shown in Fig. 2(d), when pump condition is fixed at $\Delta_{\mathrm{dc}} = 2.25 \times \Omega_{\mathrm{m1}}$ and $P_{\mathrm{d}} = -25$ dBm, the first mechanical mode is well suppressed. There are 21 comb lines, i.e., comb bandwidth of 36.8 MHz. Location of single sidebands in both spectrum in the frequency domain can be well fitted by linear function, which serve as a support for self referencing towards larger scale. It is worth noting that furthering increasing pump power in the cryogenic environment would challenge the capability of dilution refrigerator, which means towards larger scale equidistantly distributed frequency comb, room temperature setup would be preferred, and then thermal oscillation calls for consideration.

* liuyl@baqis.ac.cn
† litf@tsinghua.edu.cn

[S1] S. E. Nigg, H. Paik, B. Vlastakis, G. Kirchmair, S. Shankar, L. Frunzio, M. Devoret, R. Schoelkopf, and S. Girvin, Phys. Rev. Lett **108**, 240502 (2012).
[S2] M. Gorodetksy, A. Schliesser, G. Anetsberger, S. Deleglise, and T. J. Kippenberg, Opt. Express **18**, 23236 (2010).
[S3] X. Zhou, F. Hocke, A. Schliesser, A. Marx, H. Huebl, R. Gross, and T. J. Kippenberg, Nat. Phys. **9**, 179 (2013).
[S4] M.-A. Miri, G. D' Aguanno, and A. Alù, New J. Phys. **20**, 043013 (2018).
[S5] L. Buchmann and D. Stamper-Kurn, Phys. Rev. A **92**, 013851 (2015).
[S6] F. Marquardt, J. Harris, and S. M. Girvin, Phys. Rev. Lett. **96**, 103901 (2006).
[S7] U. Kemiktarak, M. Durand, M. Metcalfe, and J. Lawall, Phys. Rev. Lett. **113**, 030802 (2014).
[S8] L. Mercadé, K. Pelka, R. Burgwal, A. Xuereb, A. Martínez, and E. Verhagen, Phys. Rev. Lett. **127**, 073601 (2021).
[S9] Y. Hu, S. Ding, Y. Qin, J. Gu, W. Wan, M. Xiao, and X. Jiang, Phys. Rev. Lett. **127**, 134301 (2021).
